# Supplementary material for: On Exploiting Transaction Concurrency To Speed Up Blockchains
Source: arXiv:2003.06128 source file (2020-07-14)
Supplement: Supplementary file 1 [file appendix.tex]

\subsection{SQL Queries}

\begin{figure*}[!ht]
\framebox[0.99\textwidth]{
\hspace{0.1cm}
\begin{minipage}[t]{0.98\textwidth}
\begin{flushleft}
\footnotesize{\texttt{\magtxt{CREATE} \magtxt{TEMPORARY} \magtxt{FUNCTION} count\_overlaps(tx\_hashes \magtxt{ARRAY}<\magtxt{STRING}>, input\_txos \magtxt{ARRAY}<\magtxt{STRING}>) \\
\magtxt{RETURNS} \magtxt{ARRAY}<\magtxt{STRING}> \\
\magtxt{LANGUAGE} js \magtxt{AS} """ \\
\tab \magtxt{var} \blutxt{inBlockMap} = \{\}; \\
\tab \magtxt{var} \blutxt{predecessorMap} = \{\}; \\
\tab \magtxt{for}(\magtxt{var} \blutxt{i}=\grntxt{0};i<tx\_hashes.length;i++) \{ \\
\tab \tab inBlockMap[tx\_hashes[i]] = \grntxt{1}; \\
\tab \tab \magtxt{if}(predecessorMap[tx\_hashes[i]] == \viotxt{null}) predecessorMap[tx\_hashes[i]] = \magtxt{new} Set(); \\
\tab \} \\
\tab \magtxt{for}(\magtxt{var} \blutxt{i}=\grntxt{0};i<tx\_hashes.length;i++) \{ \\
\tab \tab \magtxt{if}(inBlockMap[input\_txos[i]]) \{ \\
\tab \tab \tab predecessorMap[tx\_hashes[i]].add(input\_txos[i]); \\
\tab \tab \} \\
\tab \} \\
\tab \magtxt{var} \blutxt{depth} = \grntxt{0}; \\
\tab \magtxt{var} \blutxt{numAtDepth} = []; \\
\tab \magtxt{var} \blutxt{predecessorTxs} = \magtxt{new} Set(); \\
\tab \magtxt{for}(\magtxt{var} \blutxt{i}=\grntxt{0};i<tx\_hashes.length;i++) \{ \\
\tab \tab \magtxt{for} (\magtxt{let} \blutxt{tx} \magtxt{of} predecessorMap[tx\_hashes[i]]) \{ \\
\tab \tab \tab predecessorTxs.add(tx); \\
\tab \tab \} \\
\tab \} \\
\tab \magtxt{while}(predecessorTxs.size > \grntxt{0}) \{ \\
\tab \tab \magtxt{var} \blutxt{newPredecessorTxs} = \magtxt{new} Set(); \\
\tab \tab \magtxt{for}(\magtxt{let} \blutxt{predecessorTx} \magtxt{of} predecessorTxs) \{ \\
\tab \tab \tab \magtxt{if}(inBlockMap[predecessorTx] === \grntxt{1} \&\& !(predecessorMap[predecessorTx] == \viotxt{null})) \{ \\
\tab \tab \tab \tab \magtxt{for} (\magtxt{let} \blutxt{tx} \magtxt{of} predecessorMap[predecessorTx]) \{ \\
\tab \tab \tab \tab \tab newPredecessorTxs.add(tx); \\
\tab \tab \tab \tab \} \\
\tab \tab \tab \} \\
\tab \tab \} \\
\tab \tab predecessorTxs = newPredecessorTxs; \\
\tab \tab numAtDepth[depth] = predecessorTxs.size; \\
\tab \tab depth++; \\
\tab \} \\
\tab \magtxt{var} \blutxt{numConflictingTxos} = \grntxt{0}; \\
\tab \magtxt{for}(\magtxt{var} \blutxt{i}=\grntxt{0};i<input\_txos.length;i++) \{ \\
\tab \tab \magtxt{if}(inBlockMap[input\_txos[i]] === \grntxt{1}) numConflictingTxos++; \\
\tab \} \\
\tab \magtxt{return} [Array.from(\magtxt{new} Set(tx\_hashes)).length, input\_txos.length, depth, numConflictingTxos]; \\
"""; \\
\magtxt{SELECT}  \\
\tab block\_number,  \\
\tab blocks.block\_data[OFFSET(\grntxt{0})] \magtxt{AS} num\_transactions,  \\
\tab blocks.block\_data[OFFSET(\grntxt{1})] \magtxt{AS} num\_input\_txos,  \\
\tab blocks.block\_data[OFFSET(\grntxt{2})] \magtxt{AS} max\_depth,  \\
\tab blocks.block\_data[OFFSET(\grntxt{3})] \magtxt{AS} num\_conflicting\_txos,  \\
\magtxt{FROM} ( \\
\tab \magtxt{SELECT}  \\
\tab \tab block\_number,  \\
\tab \tab count\_overlaps(ARRAY\_AGG(inputs\_merged.hash), ARRAY\_AGG(inputs\_merged.spent\_transaction\_hash))  \\
\tab \magtxt{AS}  \\
\tab \tab block\_data  \\
\tab \magtxt{FROM} ( \\
\tab \tab \magtxt{SELECT}  \\
\tab \tab \tab txs.block\_number \magtxt{AS} block\_number,  \\
\tab \tab \tab txs.hash \magtxt{AS} {\bq}hash{\bq},  \\
\tab \tab \tab inputs.spent\_transaction\_hash \magtxt{AS} spent\_transaction\_hash  \\
\tab \tab \magtxt{FROM}  \\
\tab \tab \tab {\bq}bigquery-public-data.crypto\_bitcoin.transactions{\bq} \magtxt{AS} txs,  \\
\tab \tab \tab UNNEST(inputs) \magtxt{AS} inputs \\
\tab ) \magtxt{AS} inputs\_merged \\
\tab \magtxt{GROUP} \magtxt{BY}  \\
\tab \tab block\_number  \\
\tab \magtxt{ORDER} \magtxt{BY}  \\
\tab \tab block\_number \\
) \magtxt{AS} blocks \\
}}
\end{flushleft}
\end{minipage}
}
\caption{Google BigQuery statement for Bitcoin and other blockchains with an UTXO-based data model.}
\label{fig:bitcoin_query}
\end{figure*}

\begin{figure*}[!ht]
\framebox[0.99\textwidth]{
\hspace{0.1cm}
\begin{minipage}[t]{0.98\textwidth}
\begin{flushleft}
\footnotesize{\texttt{\magtxt{CREATE} \magtxt{TEMPORARY} \magtxt{FUNCTION} components(tx\_idx \magtxt{ARRAY}<INT\grntxt{64}>, from\_addr \magtxt{ARRAY}<\magtxt{STRING}>, to\_addr \magtxt{ARRAY}<\magtxt{STRING}>, gas\_used \magtxt{ARRAY}<INT\grntxt{64}>) \\
\magtxt{RETURNS} \magtxt{ARRAY}<INT\grntxt{64}> \\
\magtxt{LANGUAGE} js \magtxt{AS} """ \\
\tab \magtxt{var} \blutxt{min\_tx\_addr} = \{\}; \magtxt{var} \blutxt{maxTx} = \grntxt{0}; \\
\tab \magtxt{for} (\magtxt{var} \blutxt{i} = \grntxt{0} ; i < tx\_idx.length; i++) \{ \\
\tab \tab \magtxt{if}(!(\grntxt{1}*tx\_idx[i] >= min\_tx\_addr[from\_addr[i]])) \{min\_tx\_addr[from\_addr[i]] = \grntxt{1}*tx\_idx[i];\} \\
\tab \tab \magtxt{if}(!(\grntxt{1}*tx\_idx[i] >= min\_tx\_addr[to\_addr[i]])) \{min\_tx\_addr[to\_addr[i]] = \grntxt{1}*tx\_idx[i];\} \\
\tab \tab \magtxt{if}(\grntxt{1}*tx\_idx[i] > maxTx) \{maxTx = \grntxt{1}*tx\_idx[i];\} \\
\tab \} \\
\tab maxTx += \grntxt{1}; \\
\tab \magtxt{var} \blutxt{min\_cl\_tx} = \magtxt{new} Array(maxTx); \magtxt{var} \blutxt{cl\_count} = \magtxt{new} Array(maxTx) \magtxt{var} \blutxt{gas\_per\_tx} = \magtxt{new} Array(maxTx); \magtxt{var} \blutxt{gas\_per\_cl} = \magtxt{new} Array(maxTx); \\
\tab \magtxt{for}(\magtxt{var} \blutxt{i} = \grntxt{0} ; i < maxTx; i++) \{ \\
\tab \tab min\_cl\_tx[i] = i; \\
\tab \tab cl\_count[i] = \grntxt{0}; \\
\tab \tab gas\_per\_cl[i] = \grntxt{0}; \\
\tab \} \\
\tab \magtxt{for} (\magtxt{var} \blutxt{i} = \grntxt{0} ; i < tx\_idx.length; i++) \{  \\
\tab \tab \magtxt{if}(!(\grntxt{1}*min\_cl\_tx[min\_tx\_addr[from\_addr[i]]] >= min\_cl\_tx[tx\_idx[i]])) \{min\_cl\_tx[tx\_idx[i]] = min\_cl\_tx[min\_tx\_addr[from\_addr[i]]];\} \\
\tab \tab \magtxt{if}(!(\grntxt{1}*min\_cl\_tx[min\_tx\_addr[to\_addr[i]]] >= min\_cl\_tx[tx\_idx[i]])) \{min\_cl\_tx[tx\_idx[i]] = min\_cl\_tx[min\_tx\_addr[to\_addr[i]]];\} \\
\tab \tab gas\_per\_tx[tx\_idx[i]] = \grntxt{1}*gas\_used[i]; \\
\tab \} \\
\tab \magtxt{for}(\magtxt{var} \blutxt{i} = \grntxt{0} ; i < maxTx; i++) \{ \\
\tab \tab cl\_count[min\_cl\_tx[i]]++; \\
\tab \tab gas\_per\_cl[min\_cl\_tx[i]] += gas\_per\_tx[i]; \\
\tab \} \\
\tab \magtxt{var} \blutxt{max\_cluster\_size} = \grntxt{0}; \magtxt{var} \blutxt{max\_cluster\_idx} = -\grntxt{1}; \magtxt{var} \blutxt{num\_unconflicted} = \grntxt{0}; \magtxt{var} \blutxt{total\_gas} = \grntxt{0}; \magtxt{var} \blutxt{unconflicted\_gas} = \grntxt{0}; \\
\tab \magtxt{for}(\magtxt{var} \blutxt{i} = \grntxt{0} ; i < cl\_count.length; i++) \{ \\
\tab \tab \magtxt{if}(cl\_count[i] > max\_cluster\_size ) \{  \\
\tab \tab \tab max\_cluster\_size = cl\_count[i];  \\
\tab \tab \tab max\_cluster\_idx = i; \\
\tab \tab \} \\
\tab \tab total\_gas += gas\_per\_tx[i]; \\
\tab \tab \magtxt{if}(cl\_count[i] === \grntxt{1}) \{ \\
\tab \tab \tab num\_unconflicted++; \\
\tab \tab \tab unconflicted\_gas += gas\_per\_tx[i]; \\
\tab \tab \} \\
\tab \} \\
\tab \magtxt{return} [max\_cluster\_size, num\_unconflicted, maxTx, gas\_per\_cl[max\_cluster\_idx], unconflicted\_gas, total\_gas, tx\_idx.length]; \\
"""; \\
\magtxt{SELECT}  \\
\tab block\_number,  \\
\tab blocks.block\_data[OFFSET(\grntxt{0})] \magtxt{AS} largest\_cluster\_num\_tx,  \\
\tab blocks.block\_data[OFFSET(\grntxt{1})] \magtxt{AS} unconflicted\_num\_tx,  \\
\tab blocks.block\_data[OFFSET(\grntxt{2})] \magtxt{AS} total\_num\_tx,  \\
\tab blocks.block\_data[OFFSET(\grntxt{3})] \magtxt{AS} largest\_cluster\_gas, \\
\tab blocks.block\_data[OFFSET(\grntxt{4})] \magtxt{AS} unconflicted\_gas, \\
\tab blocks.block\_data[OFFSET(\grntxt{5})] \magtxt{AS} total\_gas, \\
\tab blocks.block\_data[OFFSET(\grntxt{6})] \magtxt{AS} total\_traces \\
\magtxt{FROM} ( \\
\tab \magtxt{SELECT}  \\
\tab \tab block\_number,  \\
\tab \tab components(ARRAY\_AGG(transaction\_index), ARRAY\_AGG(from\_address), ARRAY\_AGG(to\_address), ARRAY\_AGG(receipt\_gas\_used)) \magtxt{AS} block\_data,  \\
\tab \magtxt{FROM} ( \\
\tab \tab \magtxt{SELECT} \\
\tab \tab \tab traces.block\_number \magtxt{AS} block\_number, \\
\tab \tab \tab traces.transaction\_index \magtxt{AS} transaction\_index,  \\
\tab \tab \tab traces.from\_address \magtxt{AS} from\_address,  \\
\tab \tab \tab traces.to\_address \magtxt{AS} to\_address, \\
\tab \tab \tab transactions.receipt\_gas\_used \magtxt{AS} receipt\_gas\_used \\
\tab \tab \magtxt{FROM}  \\
\tab \tab \tab {\bq}bigquery-public-data.ethereum\_blockchain.traces{\bq} \magtxt{AS} traces, \\
\tab \tab \tab {\bq}bigquery-public-data.ethereum\_blockchain.transactions{\bq} \magtxt{AS} transactions \\
\tab \tab \magtxt{WHERE}  \\
\tab \tab \tab traces.transaction\_index = transactions.transaction\_index  \\
\tab \tab \tab AND traces.block\_number = transactions.block\_number \\
\tab ) \\
\tab \magtxt{GROUP} \magtxt{BY}  \\
\tab \tab block\_number  \\
\tab \magtxt{ORDER} \magtxt{BY}  \\
\tab \tab block\_number \\
) \magtxt{AS} blocks \\
}}
\end{flushleft}
\end{minipage}
}
\caption{Google BigQuery statement for Ethereum and other blockchains with an account-based data model.}
\label{fig:ethereum_query}
\end{figure*}
